# Supplementary material for: Spectral Steering: Local Inverse Geometry for Frozen Diffusion Generators
Source: arXiv:2611.19572 source file (2026-11-14)
Supplement: Supplementary file 1 [file appendix_layout.tex]

\makeatletter
\newcommand{\appendixtocstart}{}
\newcommand{\printappendixcontents}{%
  \addtocontents{toc}{\protect\appendixtocstart}%
  \begingroup
    \small
    \setcounter{tocdepth}{3}%
    \setlength{\parskip}{0pt}%
    \let\appendixsavedcontentsline\contentsline
    \renewcommand{\contentsline}[4]{}%
    \renewcommand{\appendixtocstart}{\let\contentsline\appendixsavedcontentsline}%
    \@starttoc{toc}%
  \endgroup
}
\newcommand{\setupappendixlayout}{%
  \setlength{\@fptop}{0pt}%
  \renewcommand{\topfraction}{0.95}%
  \renewcommand{\bottomfraction}{0.90}%
  \renewcommand{\textfraction}{0.05}%
  \renewcommand{\floatpagefraction}{0.65}%
  \setcounter{topnumber}{4}\setcounter{bottomnumber}{3}\setcounter{totalnumber}{6}%
  \setlength{\floatsep}{8pt plus 2pt minus 2pt}%
  \setlength{\textfloatsep}{10pt plus 2pt minus 2pt}%
  \setlength{\intextsep}{8pt plus 2pt minus 2pt}%
  \setlength{\@fpsep}{8pt plus 2pt}%
  \AddToHook{cmd/section/before}{\Needspace{5\baselineskip}}%
  \AddToHook{cmd/subsection/before}{\Needspace{4\baselineskip}}%
  \AddToHook{cmd/subsubsection/before}{\Needspace{4\baselineskip}}%
}
\makeatother
